# Supplementary material for: Rethinking Vision Transformers for MobileNet Size and Speed
Source: arXiv:2212.08059 source file (2023-09-04)
Supplement: Supplementary file 5 [file supp_3_searchalpha.tex]

\begin{table}[h]
\centering
% \small
\caption{Analysis of the $\alpha_{latency}$ and $\alpha_{size}$ in search algorithm.}\label{tab:search_alpha}
% \label{tab_alpha}
\resizebox{1\linewidth}{!}{
\begin{tabular}{ccccc}
\toprule
$\alpha_{latency}$ & $\alpha_{size}$ & Params (M) & Latency & Top-1 (\%) \\
\hline
1.0       & 1.0    &    3.5    &   1.1 ms     &    77.0   \\
0.5       & 1.0    &    3.5    &  1.3 ms      &  77.3     \\
\hline
\rowcolor[gray]{0.92}
1.0       & 0.5    & 3.5    & 0.9 ms    & 75.7  \\
\bottomrule
\end{tabular}
}
\end{table}
% \end{wraptable}
