# Supplementary material for: Rethinking Vision Transformers for MobileNet Size and Speed
Source: arXiv:2212.08059 source file (2023-09-04)
Supplement: Supplementary file 8 [file supp_2_downstream.tex]

\begin{table*}[]
\centering
% \small
\caption{
\textbf{Object detection \&
instance segmentation} on MS COCO 2017. We benchmark on Mask RCNN pipeline. \dagger~refers to the results obtained from the enhanced training recipe. }
% \resizebox{1.0\linewidth}{!}{
% \begin{tabular}{c|c|cccccc}
% \toprule
% \multirow{2}{*}{Backbone} & \multirow{2}{*}{Params (M)} & \multicolumn{6}{c}{Detection \& Instance Segmentation}  \\ \cline{3-8}
%                           &                         & AP$^{box}$    & AP$^{box}_{50}$   & AP$^{box}_{75}$   & AP$^{mask}$    & AP$^{mask}_{50}$   & AP$^{mask}_{75}$      \\
%                           \hline
%                           \hline
% ResNet18                  &     11.7        & 34.0   & 54.0    & 36.7    & 31.2   & 51.0    & 32.7       \\
% PoolFormer-S12            &     12.0          & 37.3   & 59.0    & 40.1    & 34.6   & 55.8    & 36.9        \\
% EfficientFormer-L1        &     12.3              & 37.9   & 60.3    & 41.0    & 35.4   & 57.3    & 37.3       \\
% EfficientFormerV2-S2      &     12.6              &  38.9  &  60.3   & 42.4  &    35.5    &   57.2      &  37.8      \\
% \rowcolor[gray]{0.92}
% EfficientFormerV2-S2\dagger     &     12.6              &  43.4  &  65.4   & 47.5  &    39.5    &   62.4      &  42.2      \\
% \hline
% ResNet50                  &      25.5           & 38.0   & 58.6    & 41.4    & 34.4   & 55.1    & 36.7      \\
% PoolFormer-S24            &     21.0            & 40.1   & 62.2    & 43.4    & 37.0   & 59.1    & 39.6     \\
% Swin-T                    &     29.0              & 42.2   & 64.4    & 46.2    & 39.1   & 64.6    & 42.0      \\
% % PVTv2-B2                  &                         & 45.3   & 67.1    & 49.6    & 41.2   & 64.2    & 44.4    \\
% % Twins-SVT-S               &                         & 43.4   & 66.0    & 47.3    & 40.3   & 63.2    & 43.4      \\
% EfficientFormer-L3        &         31.3     & 41.4   & 63.9    & 44.7    & 38.1   & 61.0    & 40.4      \\
% % CSwin-T                   &                         & 46.7   & 68.6    & 51.3    & 42.2   & 65.6    & 45.4     \\
% EfficientFormerV2-L       &       26.1      & 42.4   &  64.2  &  46.7   &  38.7   &  61.1   & 41.6           \\
% \rowcolor[gray]{0.92}
% EfficientFormerV2-L\dagger      &       26.1      & 44.7   &  66.3  &  48.8   &  40.4   &  63.5   & 43.2           \\
% \bottomrule
% \end{tabular}

\begin{tabular}{c|c|cccccc|c}
\toprule
\multirow{2}{*}{Backbone} & \multirow{2}{*}{Params (M)} & \multicolumn{6}{c}{Detection \& Instance Segmentation} & \multicolumn{1}{c}{Semantic}  \\ \cline{3-9}
                          &                         & AP$^{box}$    & AP$^{box}_{50}$   & AP$^{box}_{75}$   & AP$^{mask}$    & AP$^{mask}_{50}$   & AP$^{mask}_{75}$   & mIoU   \\
                          \hline
                          \hline
ResNet18                  &     11.7        & 34.0   & 54.0    & 36.7    & 31.2   & 51.0    & 32.7   & 32.9   \\
PoolFormer-S12            &     12.0          & 37.3   & 59.0    & 40.1    & 34.6   & 55.8    & 36.9     & 37.2  \\
EfficientFormer-L1        &     12.3              & 37.9   & 60.3    & 41.0    & 35.4   & 57.3    & 37.3   &  38.9  \\
% EfficientFormerV2-S2      &     12.6              &  38.9  &  60.3   & 42.4  &    35.5    &   57.2      &  37.8   &   \\
\rowcolor[gray]{0.92}
EfficientFormerV2-S2     &     12.6              &  43.4  &  65.4   & 47.5  &    39.5    &   62.4      &  42.2   & 42.4  \\
\hline
ResNet50                  &      25.5           & 38.0   & 58.6    & 41.4    & 34.4   & 55.1    & 36.7  &  36.7  \\
PoolFormer-S24            &     21.0            & 40.1   & 62.2    & 43.4    & 37.0   & 59.1    & 39.6  &  40.3 \\
Swin-T                    &     29.0              & 42.2   & 64.4    & 46.2    & 39.1   & 64.6    & 42.0   & 41.5  \\
% PVTv2-B2                  &                         & 45.3   & 67.1    & 49.6    & 41.2   & 64.2    & 44.4    \\
% Twins-SVT-S               &                         & 43.4   & 66.0    & 47.3    & 40.3   & 63.2    & 43.4      \\
EfficientFormer-L3        &         31.3     & 41.4   & 63.9    & 44.7    & 38.1   & 61.0    & 40.4   &  43.5 \\
% CSwin-T                   &                         & 46.7   & 68.6    & 51.3    & 42.2   & 65.6    & 45.4     \\
% EfficientFormerV2-L       &       26.1      & 42.4   &  64.2  &  46.7   &  38.7   &  61.1   & 41.6    &       \\
\rowcolor[gray]{0.92}
EfficientFormerV2-L      &       26.1      & 44.7   &  66.3  &  48.8   &  40.4   &  63.5   & 43.2     &   45.2   \\
\bottomrule
\end{tabular}

% }
\label{tab:coco_improved}
\end{table*}

% \begin{table}[]
% \centering
% % \small
% \caption{\textbf{Semantic segmentation} on ADE20K. EfficientFormerV2 models are integrated as feature encoder in Semantic FPN. \dagger~refers to the results obtained from the enhanced training recipe. }
% \begin{tabular}{c|c|c}
% \toprule
% Backbone             & Params (M) & mIoU \\
% \hline
% ResNet18             & 11.7 & 32.9 \\
% PoolFormer-S12       & 12.0 & 37.2 \\
% EfficientFormer-L1   & 12.3 & 38.9 \\
% EfficientFormerV2-S2 & 12.6 & 39.5 \\
% \rowcolor[gray]{0.92}
% EfficientFormerV2-S2\dagger & 12.6 & 42.4 \\
% \hline
% ResNet50             & 25.5 & 36.7 \\
% PoolFormer-S24       & 21.0 & 40.3 \\
% EfficientFormer-L3   & 31.3 & 43.5 \\
% % EfficientFormerV2-L & 26.1 & 39.7 \\
% \rowcolor[gray]{0.92}
% EfficientFormerV2-L\dagger & 26.1 & 45.2 \\
% \bottomrule
% \end{tabular}
% \label{tab:ade20k_improved}
% \end{table}
