# Supplementary material for: Rethinking Vision Transformers for MobileNet Size and Speed
Source: arXiv:2212.08059 source file (2023-09-04)
Supplement: Supplementary file 12 [file supp_network_architecture.tex]

\begin{table*}[ht]
% \centering
\caption{Architecture details of EfficientFormerV2.}
\label{tab:achitecture}
\begin{tabular}{c|c|c|c|c|c|c|c}
\toprule
\multirow{2}{*}{Stage} & \multirow{2}{*}{Resolution} & \multirow{2}{*}{Type} & \multirow{2}{*}{Config} & \multicolumn{4}{c}{EfficientFormerV2}                                   \\ \cline{5-8}
                       &                             &                       &                         & S0                & S1                & S2            & L               \\
                       \hline
\multirow{4}{*}{stem}  & \multirow{2}{*}{$\frac{H}{2}\times \frac{W}{2}$}         & \multirow{2}{*}{\texttt{Conv}} & Kernel, Stride           & $3\times 3$, $2$            & $3\times 3$, $2$            & $3\times 3$, $2$        & $3\times 3$, $2$          \\ \cline{4-8}
                       &                             &                       & N, C                    & $1$, $16$             & $1$, $16$             & $1$, $16$         & $1$, $20$           \\ \cline{2-8}
                       & \multirow{2}{*}{$\frac{H}{4}\times \frac{W}{4}$}         & \multirow{2}{*}{\texttt{Conv}} & Kernel, Stride           & $3\times 3$, $2$            & $3\times 3$, $2$            & $3\times 3$, $2$        & $3\times 3$, $2$          \\ \cline{4-8}
                       &                             &                       & N, C                    & $1$, $32$             & $1$, $32$             & $1$, $32$         & $1$, $40$           \\
                       \hline
\multirow{2}{*}{1}     & \multirow{2}{*}{$\frac{H}{4}\times \frac{W}{4}$}         & \multirow{2}{*}{\texttt{FFN}}  & N, C                    & $2$, $32$             & $3$, $32$             & $4$, $32$         & $5$, $40$           \\ \cline{4-8}
                       &                             &                       & E                       & {[}$4,4${]}         & {[}$4,4,4${]}       & {[}$4,4,4,4${]} & {[}$4,4,4,4,4${]} \\
                       \hline
\multirow{2}{*}{2}     & \multirow{2}{*}{$\frac{H}{8}\times \frac{W}{8}$}         & \multirow{2}{*}{\texttt{FFN}}  & N, C                    & $2, 48$             & $3, 48$             & $4, 64$         & $5, 80$           \\ \cline{4-8}
                       &                             &                       & E                       & {[}$4,4${]}         & {[}$4,4,4${]}       & {[}$4,4,4,4${]} & {[}$4,4,4,4,4${]} \\
                       \hline
\multirow{3}{*}{3}     & \multirow{3}{*}{$\frac{H}{16}\times \frac{W}{16}$}        & \multirow{2}{*}{\texttt{FFN}}  & N, C                    & $6, 96$             & $9, 120$            & $12, 144$       & $15, 192$         \\  \cline{4-8}
                       &                             &                       & E                       & {[}$4,3,3,3,4,4${]} & {[}$4(\times5),3(\times4)${]}     & {[}$4(\times6),3(\times6)${]} & {[}$4(\times8),3(\times7)${]}   \\
                      \cline{3-8}
                       &                             & \texttt{MHSA}                  & N                       & $2$                 & $2$                 & $4$             & $6$               \\
                       \hline
\multirow{3}{*}{4}     & \multirow{3}{*}{$\frac{H}{32}\times \frac{W}{32}$}        & \multirow{2}{*}{\texttt{FFN}}  & N, C                    & $4, 176$            & $6, 224$            & $8, 288$        & $10, 384$         \\ \cline{4-8}
                       &                             &                       & E                       & {[}$4,3,3,4${]}     & {[}$4,4,3,3,4,4${]} & {[}$4(\times4),3(\times4)${]} & {[}$4(\times6), 3(\times4)${]}  \\
                       \cline{3-8}
                       &                             & \texttt{MHSA}                  & N                       & $2$                 & $2$                 & $4$             & $6$  \\
                       \bottomrule
\end{tabular}
\end{table*}
